# Supplementary material for: Herding of proteins by the ends of shrinking polymers
Source: arXiv:2112.07757 source file (2022-09-08)

(a)

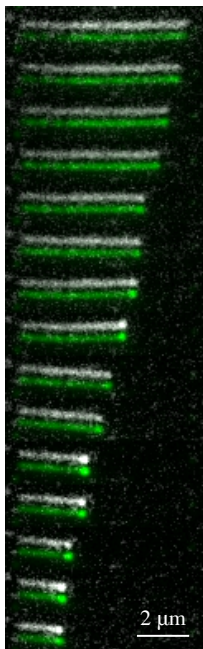

(b)

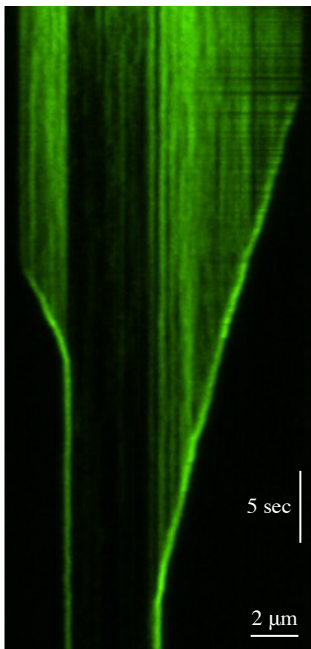

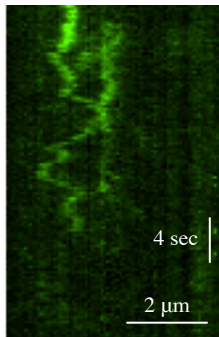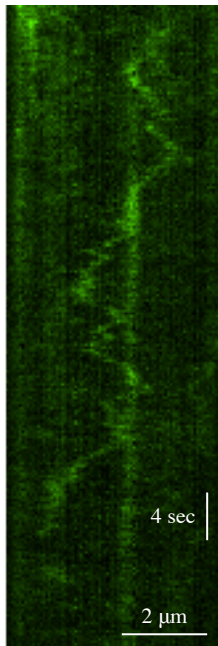

Supplement: Supplementary file 2 [file Figure_S2_and_S3-SuppExperiments.pdf]
